# Supplementary material for: BBQ-Networks: Efficient Exploration in Deep Reinforcement Learning for Task-Oriented Dialogue Systems
Source: arXiv:1608.05081 source file (2017-11-23)
Supplement: Supplementary file 1 [file appendix.tex]

\section{Minimizing the KL Divergence between two Univariate Gaussians}
\label{sec:KL}

\section{Dialog System Architecture}
\label{sec:dialogdetail}

\section{Learned Variational Parameters}
\label{sec:variational-parameters}
\begin{figure}[t!]
	\centering
	\begin{subfigure}[b]{0.33\linewidth}
  		\raggedleft
		\includegraphics[scale=.31]{img/mean_distribution.png}
		\caption{means $\mu_q$ }
		\label{fig:mean-heatmap}
	\end{subfigure}~
	\begin{subfigure}[b]{0.33\textwidth}
  		\centering
		\includegraphics[scale=.31]{img/variance_distribution.png}
		\caption{standard deviations $\sigma_q$}
		\label{fig:sigma-heatmap}
	\end{subfigure}~
	\begin{subfigure}[b]{0.33\textwidth}
		\raggedright
		\includegraphics[scale=.30]{img/signal_to_noise.png}
		\caption{signal to noise ratios $|\mu_q|/|\sigma_q|$}
		\label{fig:signal-to-noise-heatmap}
	\end{subfigure}
\caption{Histograms of the the means (a), standard deviations (b), and signal to noise ratios (c), among the weights in the network. Early in training, the regularizer $\mbox{KL} [q(\boldsymbol{w}|\theta) || p(\boldsymbol{w}]$ has higher weight in the cost function, keeping weights close to the prior distribution, resulting in high exploration, as the experience replay buffer fills, many weights  }
\label{}
\end{figure}

\section{Deep Q Network Architecture}
\label{sec:q-network}

\begin{figure*}[t!]
	\centering
	\begin{subfigure}[b]{0.5\textwidth}
  		\centering
		\includegraphics[scale=.4]{img/DQN.png}
        \caption{The DQN shares hidden layers among actions, making for efficient inference of $\argmax_a Q(s,a)$}
		\label{fig:dqn-arch} 
	\end{subfigure}~
	\begin{subfigure}[b]{0.5\textwidth} 
  		\centering
		\includegraphics[scale=.4]{img/DQN-mask.png}
		\caption{For any training example, loss is calculated only for the corresponding action $a$.}
		\label{fig:dqn-mask}
	\end{subfigure}
\caption{}
\label{fig:dqn}
\end{figure*}
