# Supplementary material for: BBQ-Networks: Efficient Exploration in Deep Reinforcement Learning for Task-Oriented Dialogue Systems
Source: arXiv:1608.05081 source file (2017-11-23)
Supplement: Supplementary file 2 [file dqn-appendix.tex]

An RL agent navigates a Markov decision process (MDP), 
interacting with its environment 
over a sequence of discrete steps. 
At each step $t$, the agent observes the current state $s_t \in \mathcal{S}$, and chooses some action $a_t \in \mathcal{A}$ according to a policy $\pi$.
The agent then receives reward $r_{t}$ 
and observes new state $s_{t+1}$, 
continuing the cycle until the episode terminates. 
Here, $\mathcal{S}$ represents the set of all possible states, 
$\mathcal{A}$ defines the space of possible actions 
and the policy $\pi: \mathcal{S} \rightarrow \mathcal{A}$ maps states onto actions.
In this work, we assume actions to be discrete and $|\mathcal{A}|$ to be finite.
Under a policy $\pi$ and in state $s$ the \emph{value}
of action $a$ is the expected cumulative discounted reward (also known as \emph{return}):
$$Q^{\pi}(s,a) = \mathbbm{E}_{\pi}\left[ \sum_{i=0}^T \gamma^i r_{t+i} | s_t =s, a_t=a \right]\,$$
where $\gamma$ is a discount factor.
An optimal policy is one whose $Q$-function uniformly dominates others. Its value function, called the \emph{optimal value function}, is denoted $Q^*$~\cite{sutton1998reinforcement}.
Owing to large state spaces, most practical reinforcement learners approximate the Q function by some parameterized model $Q(s,a;\theta)$ among which deep neural networks have become especially popular.

Given the optimal value function $Q^*$,
at any time-step $t$, the optimal move is for the agent to choose action $a^* = \argmax_a Q^*(s,a)$. 
Thus, learning an optimal policy can be reduced to learning the optimal value function.
For toy problems, where an environment can be fully explored, 
we can maintain an estimate of the Q function 
as a table of values, with rows indexing each state and columns for each action.
In practice, the number of states may be intractably large, 
and the sample complexity of exploration can 
grow at least linearly
with the number of states $|S|$ and the size of the action space $|\mathcal{A}|$.
Thus, most practical reinforcement learners approximate the Q function by some parameterized model $Q(s,a;\theta)$,
among which deep neural networks have become especially popular.

The definition of return specifies a recursion: 
the value of the current state, action pair $(s,a)$, depends upon the expected value of the successor state $s_{t+1}$ and the action chosen in that state:
$$Q(s_t,a_t) = r_{t} + \gamma \max_{a'} Q(s_{t+1}, a')\,.$$
For a fixed policy, the value function can be iteratively improved
by approximate value iteration.
We represent experiences as tuples $(s_t, a_t, r_{t}, s_{t+1})$.
In Q-learning, we aim to improve the value function (and, in turn, the greedy policy) by minimizing the squared error between the current prediction and the one step look-ahead prediction
\begin{equation}
\mathcal{L}(\theta_t) = 
\mathbbm{E}
% _{(s_t,a_t, r_t, s_{t+1}) \sim \rho(\cdot)}
\left[
(y_t - Q(s_t, a_t; \theta_t))^2 
\right]
\end{equation}
for $y_t = r_t + \gamma \max_{a'} Q(s_{t+1}, {a'}; \theta_{t})$. 
% and for $\rho(\cdot)$ denoting the joint distribution of experiences under the current policy.
Traditionally, the Q-function is trained by stochastic approximation, estimating the loss on each experience as it is encountered, yielding the update:
\begin{equation}
\begin{split}
\theta_{t+1} \gets & \theta_t + \alpha (
%r_{t} + \gamma \max_{a'} Q(s_{t+1}, a'; \theta_t) 
y_t - Q(s_t,a_t;\theta_t)) \nabla Q(s_t,a_t;\theta_t).
\end{split}
\end{equation}

A few tricks improve the effectiveness of DQNs. 
First, \emph{experience replay} maintains a buffer of experiences, 
training off-policy on randomly selected mini-batches~\cite{lin1992self,mnih15human}. 
Second, it's common to periodically cache DQN parameters parameters, 
using the stale parameters to compute the training targets $y_t$.

Other techniques such as double deep Q-learning~\cite{van2015deep} and prioritized experience replay~\cite{schaul2015prioritized} 
%(a form of importance sampling)
appear effective for learning the Q-function.
% In contrast, our focus here is about generating ``useful'' replay experience---the issue of efficient exploration.  
For simplicity and because these techniques are straightforward to combine with ours, 
we build on the basic DQN model and focus on the issue of exploration.

In order to expose the agent to a rich set of experiences, one must employ a strategy for exploration.
Most commonly in the DQN literature, researchers use the $\epsilon$-greedy exploration heuristic.
In this work, we improve upon greedy exploration strategies by using uncertainty information (in the predicted Q values) to make more intelligent exploration choices.
