# Supplementary material for: BBQ-Networks: Efficient Exploration in Deep Reinforcement Learning for Task-Oriented Dialogue Systems
Source: arXiv:1608.05081 source file (2017-11-23)
Supplement: Supplementary file 3 [file bbb-appendix.tex]

We now introduce Bayes-by-Backprop~\cite{blundell2015weight}, a method for extracting uncertainty information from neural networks by maintaining a probability distribution over the weights in the network.
We confine the present discussion to multilayer perceptrons (MLPs), i.e., 
feedforward neural networks composed entirely of fully connected layers, without recurrent connections. 
A standard MLP for regression models 
$P(\boldsymbol{y}|\boldsymbol{x}, \boldsymbol{w})$, 
parameterized by weights $\boldsymbol{w} = \{W_l, b_l\}_{l=1}^{L}$.
MLPs have the simple architecture:
$$\boldsymbol{\hat{y}}= W_L \cdot \phi(W_{L-1} \cdot ... \cdot \ \phi(W_1 \cdot \boldsymbol{x} + b_1) + ... + b_{L-1}) + b_L$$
for a network with $L$ layers ($L-1$ hidden) and activation function $\phi$ (commonly sigmoid, tanh, or rectified linear unit (ReLU). 
% For a regression task, the topmost layer typically does not apply a nonlinearity.

In standard neural network training, 
we learn the weights $\boldsymbol{w}$ 
given a dataset $\mathcal{D} = \{ \boldsymbol{x}_i,
\boldsymbol{y}_i
\}_{i=1}^N$ by maximum likelihood estimation (MLE), 
using some variant of stochastic gradient descent:  
$\boldsymbol{w}^{MLE} = \argmax_{\boldsymbol{w}} \log p(\mathcal{D}|\boldsymbol{w})$.
% 						& = \argmax_{\boldsymbol{w}} \sum_i \ln p(\boldsymbol{y}_i | \boldsymbol{x}_i, \boldsymbol{w}) 
Frequently, we regularize models by placing priors on the parameters $\boldsymbol{w}$. 
The resulting optimization seeks the maximum a posteriori (MAP) assignment $\boldsymbol{w^{MAP}} = \argmax_{\boldsymbol{w}} \log p(\boldsymbol{w}|\mathcal{D})$.
% We can express this via Bayes rule as a function of both $p(\mathcal{D}|\boldsymbol{w})$ and $p(\boldsymbol{w})$.
This yields $\ell_2^2$ regularization 
for Gaussian prior or $\ell_1$ regularization for Laplace prior:
\begin{equation}
\begin{split}
\boldsymbol{w}^{MAP} & = \argmax_{\boldsymbol{w}} \log p(\boldsymbol{w}|\mathcal{D})\\
% 					& = \argmax_{w} \ln p(\mathcal{D}|\boldsymbol{w})P(\boldsymbol{w}) \\
					& = \argmax_{w} \ln p(\mathcal{D}|\boldsymbol{w}) + \ln p(\boldsymbol{w}). 
\end{split}
\end{equation}

Both MLE and MAP assignments produce point estimates of $\boldsymbol{w}$, and thus capture only the mode of the predictive distribution, 
% yielding a deterministic mapping function $f: \mathcal{X} \rightarrow \mathcal{Y}$. 
But to enable efficient exploration, 
we prefer a model that can quantify uncertainty.
Thus, we consider a Bayesian treatment of neural networks, 
learning a full posterior distribution 
%over the weights 
$p(\boldsymbol{w}|\mathcal{D})$.

Problematically, $p(\boldsymbol{w}|\mathcal{D})$ may be intractable.
The weights may be arbitrarily correlated and the joint distribution might be of arbitrary complexity, 
and thus difficult both to learn and to sample from.
So we approximate the potentially intractable posterior by a variational distribution $q(\boldsymbol{w}|\theta)$.
In this work,
we choose $q$ to be Gaussian with diagonal covariance.
Thus, we sample each weight $w_i$ from a univariate Gaussian distribution parameterized by mean $\mu_i$ and standard deviation $\sigma_i$. 
To ensure that all $\sigma_i$ remain strictly positive,
we parameterize $\sigma_i$  
by the softplus function $\sigma_i = \log (1 + \mbox{exp}(\rho_i))$, 
giving variational parameters $\theta = \{(\mu_i, \rho_i) \}_{i=1}^{D}$ for $D$-dimensional weight vector $\boldsymbol{w}$. 

Note that the true posterior is both multi-modal (owing to symmetry among the nodes) and intractable. There is no reason to believe that the true posterior exhibits conditional independence between every pair of two weights regardless of the values taken by the others. So this is only an approximation in a very narrow sense. Nonetheless, it proves useful in practice.

We learn these parameters by minimizing the Kullback-Liebler (KL) divergence 
between the variational
approximation $q(\boldsymbol{w}|\theta)$ 
and the posterior $p(\boldsymbol{w}|\mathcal{D})$
\begin{equation}
\begin{split}
\theta^* & = \mbox{argmin}_{\theta} \mbox{KL} 
[q(\boldsymbol{w}|\theta) || p(\boldsymbol{w}| \mathcal{D})]\\
& = \mbox{argmin}_{\theta} 
\int %_{-\infty}^{\infty} 
q(\boldsymbol{w}|\theta) 
\log \frac{q(\boldsymbol{w}|\theta)}{p(\boldsymbol{w})p(\mathcal{D}|\boldsymbol{w})}
\mbox{d$\boldsymbol{w}$}\\
& = \mbox{argmin}_{\theta} \mbox{KL}[q(\boldsymbol{w}|\theta) || p(w)]
- \mathbbm{E}_{q(\boldsymbol{w}|\theta)}
[\log p(\mathcal{D}|\boldsymbol{w})].
\end{split}
\end{equation}
The expression minimized is termed by~\cite{hinton1993keeping} 
the \emph{variational free energy}
$$\mathcal{F} = \mbox{KL}[q(\boldsymbol{w}|\theta) || p(w)]
- \mathbbm{E}_{q(\boldsymbol{w}|\theta)}
[\ln p(\mathcal{D}|\boldsymbol{w})].$$
The term on the left term penalizes distance between the variational posterior $q(\boldsymbol{w}|\theta)$
and the prior $p(w)$. 
Specifically, the KL divergence measures the amount of information (measured in nats) 
that are lost when $p(\boldsymbol{w})$ is used to approximate $q(\boldsymbol{w}|\theta)$.
Therefore, \namecite{hinton1993keeping} describe this term as a penalty on the description length of weights.
Assuming a Gaussian predictive distribution, the rightmost term is simply the expected square loss.
Sampling from $q$, our cost function is
$f(\mathcal{D}, \theta) =
\log q(\boldsymbol{w}|\theta) - \log p(\boldsymbol{w}) - \log p(\mathcal{D}|\boldsymbol{w})$. 
When $q(\boldsymbol{w}|\theta)$ and $p(\boldsymbol{w})$ are both parameterized as univariate Gaussian distributions, 
their distance is minimized by setting $\mu_q = \mu_p$ for every setting of the variances, and by setting the standard deviations $\sigma_q = \sigma_p$ for any setting of the means $\mu_q$ and $\mu_p$. 
%[Proof in Appendix A] Add appendix for submission?

% \subsection{Minimising Loss By Stochastic Gradient Variational Bayes}
% Owing to this variational approach, 
% we can learn a probabilistic model without sacrificing the efficiency of gradient-based training.
We can learn the variational parameters $\theta$ 
by gradient descent, using the reparametrization trick popularized by \namecite{kingma2013auto}.
In short, 
we want to differentiate the loss with respect to the  variational parameters $\theta$, 
but the loss depends upon the random vector $\boldsymbol{w} \sim q(\boldsymbol{w}|\theta)$.
We can overcome this problem by expressing $\boldsymbol{w}$ as a deterministic function of $\theta$, $g(\boldsymbol{\eta}, \theta)$,
where $\boldsymbol{\eta}$ is a random vector.
When we choose $g$ and noise distribution $p(\boldsymbol{\eta})$ such that $p(\boldsymbol{\eta}) d\boldsymbol{\eta} = q(\boldsymbol{w}|\theta) d\boldsymbol{w}$,
we can express our optimization objective equivalently as an expectation over $\eta$.
In our case, we take $\boldsymbol{\eta}$ to be a noise vector drawn from $D$-dimensional standard  normal $\mathcal{N}(\boldsymbol{0},I)^D$.
Thus $\boldsymbol{w} = g(\boldsymbol{\eta},\theta)= \boldsymbol{\mu} + \log(1 + \mbox{exp}(\boldsymbol{\rho})) \odot \boldsymbol{\eta}$, where $\odot$ is the element-wise product.

For any given value of $\eta$ our loss is differentiable with respect to the variational parameters.
We can then proceed with backpropagation, treating $\boldsymbol{\eta}$ as a noise input
sampled for each batch. 
Thus, we minimize the loss by stochastic gradient descent, 
using a single Monte Carlo sample 
$\boldsymbol{\eta} \sim p(\boldsymbol{\eta})$ at each iteration.
In our case, we take $\boldsymbol{\eta}$ to be a noise vector drawn from isotropic standard  normal $\mathcal{N}(0,I)^D$.
% Thus $\boldsymbol{w} = g(\boldsymbol{\eta},\theta)= \boldsymbol{\mu} + \log(1 + \mbox{exp}(\boldsymbol{\rho})) \odot \boldsymbol{\eta}$, where $\odot$ is the element-wise product.
% For our work, the optimization objective becomes:
% \begin{equation}
% f(\boldsymbol{w}, \theta) =
% \log q(\boldsymbol{w}|\theta) - \log p(\boldsymbol{w}) - p(\mathcal{D}|\boldsymbol{w})
% \end{equation}
